# Supplementary material for: Provably Safeguarding a Classifier from OOD and Adversarial Samples: an Extreme Value Theory Approach
Source: arXiv:2501.10202 source file (2025-01-17)
Supplement: Supplementary file 1 [file tab_ood_SM.tex]

\begin{table}
    \centering
    \caption{Comparative performance of SPADE (with teacher ResNet) against MSP, ODIN, MDS and KNN:  detection of near OOD, far OOD and adversarial examples on \CifarC\ and \CifarD\ using  AUROC ($\uparrow$) and FPR95 ($\downarrow$) indicators.
    Statistically significantly best performances are in bold.}
    \resizebox{0.75\linewidth}{!}{\begin{tabular}{cccccccc}
    \toprule 
         & & \multicolumn{2}{c}{\textbf{Near OOD}} & \multicolumn{2}{c}{\textbf{Far OOD}} & \multicolumn{2}{c}{\textbf{Adversarial}}  \\
         && \textbf{AUC} $\uparrow$ & \textbf{FPR95} $\downarrow$ &\textbf{AUC} $\uparrow$ & \textbf{FPR95} $\downarrow$ & \textbf{AUC} $\uparrow$ & \textbf{FPR95} $\downarrow$  \\
         \midrule 
         \parbox[t]{2mm}{\multirow{5}{*}{\rotatebox[origin=c]{90}{\CifarD}}} 
         &MSP \citepalias{hendrycks2018baseline}&87.68&53.54&91.00&31.43&81.96&78.76\\
         &ODIN \citepalias{liang2020enhancing}&80.25&84.49&87.21&60.89&-&-\\
         &MDS \citepalias{lee2018simple}&86.72&46.23&90.20&30.31&81.54&69.14\\
         &KNN \citepalias{pmlr-v162-sun22d} &90.70&\textbf{34.54}&93.11&23.88&85.79&\bf 54.21\\[0.2mm]\cmidrule{2-8} 
         &\bf \XX&\textbf{90.85}&34.74&\textbf{93.44}&\textbf{22.97}&\bf 86.10&54.43\\
         \midrule
         \parbox[t]{2mm}{\multirow{5}{*}{\rotatebox[origin=c]{90}{\CifarC}}} &MSP \citepalias{hendrycks2018baseline}&80.14&\textbf{55.23}&77.34&59.77&83.46&\bf 50.50\\
         &ODIN \citepalias{liang2020enhancing} &79.86&58.03&78.98&59.34&-&-\\
         &MDS \citepalias{lee2018simple} &58.68&84.22&70.65&72.04&60.27&82.89\\
         &KNN \citepalias{pmlr-v162-sun22d}&80.32&61.33&\textbf{82.64}&53.47&83.72&56.00\\[0.2mm] \cmidrule{2-8}
         &\bf  
\XX&\textbf{80.70}&59.36&81.95&\textbf{53.27}&\bf 84.50&52.72\\
         \bottomrule
         \end{tabular}}
    \label{tab:ood_detection_sm}
\end{table}
